# Supplementary material for: Trends in Integration of Vision and Language Research: A Survey of Tasks, Datasets, and Methods
Source: arXiv:1907.09358 source file (2021-12-31)
Supplement: Supplementary file 1 [file appendix.tex]

\nomenclature[A]{\textbf{ADAM}}{ADAptive Moment estimation}
\nomenclature[A]{\textbf{AI}}{Artificial Intelligence}
\nomenclature[A]{\textbf{AMEM}}{Attention MEMory}
\nomenclature[A]{\textbf{AMT}}{Amazon Mechanical Turk}
\nomenclature[A]{\textbf{ANetCap}}{ActivityNet Captions}
\nomenclature[A]{\textbf{AREL}}{Adversarial REward Learning}
\nomenclature[A]{\textbf{AVSD}}{Audio Visual Scene-aware Dialog}

\nomenclature[A]{\textbf{BDD}}{Berkeley Deep Drive}
\nomenclature[A]{\textbf{BDD-X}}{Berkeley Deep Drive eXplanation}
\nomenclature[A]{\textbf{BERT}}{Bidirectional Encoder Representations from Transformers}
\nomenclature[A]{\textbf{BiLSTM}}{Bidirectional LSTM}
\nomenclature[A]{\textbf{BLEU}}{BiLingual Evaluation Understudy}
\nomenclature[A]{\textbf{BRNN}}{Bidirectional Recurrent Neural Network}

\nomenclature[A]{\textbf{CIDEr}}{Consensus based Image Description Evaluation}
\nomenclature[A]{\textbf{CLEVR}}{Compositional Language and Elementary Visual Reasoning}
\nomenclature[A]{\textbf{CLEVR-CoGenT}}{CLEVR Compositional Generalization Test}
\nomenclature[A]{\textbf{CLID}}{Cross-Lingual Image Description}
\nomenclature[A]{\textbf{CMM}}{Cascaded Mutual Modulation}
\nomenclature[A]{\textbf{CMRE}}{Cross-Modal Relationship Extractor}
\nomenclature[A]{\textbf{CNN}}{Convolutional Neural Networks}
\nomenclature[A]{\textbf{COG}}{Configurable Visual Question and Answer}
\nomenclature[A]{\textbf{CoAtt-GAN}}{Co-Attention GAN}
\nomenclature[A]{\textbf{CorefNMN}}{Coreference Neural Module Networks}
\nomenclature[A]{\textbf{CUB}}{Caltech-UCSD Birds}

\nomenclature[A]{\textbf{DII}}{Descriptions of Images-in-Isolation}
\nomenclature[A]{\textbf{DIS}}{Descriptions of Images-in-Sequence}

\nomenclature[A]{\textbf{EVE}}{Explainable Visual Entailment}

\nomenclature[A]{\textbf{FAST}}{Frontier Aware Search with backTracking}
\nomenclature[A]{\textbf{FiLM}}{Feature-wise Linear Modulation}
\nomenclature[A]{\textbf{FID}}{Fr\'{e}chet Inception Distance}

\nomenclature[A]{\textbf{GAN}}{Generative Adversarial Network}
\nomenclature[A]{\textbf{GAWWN}}{Generative Adversarial What-Where Network}
\nomenclature[A]{\textbf{GGCN}}{Gated Graph Convolutional Network}
\nomenclature[A]{\textbf{GNN}}{Graph Neural Network}
\nomenclature[A]{\textbf{GRU}}{Gated Recurrent Unit}
\nomenclature[A]{\textbf{GVF}}{Global Visual Features}
\nomenclature[A]{\textbf{GQA}}{General Question Answering}

\nomenclature[A]{\textbf{HCIAE-NP-ATT}}{History-Conditioned Image Attentive Encoder n-pair self-ATTentive}
\nomenclature[A]{\textbf{HRE}}{Hierarchical Recurrent Encoder}
\nomenclature[A]{\textbf{HREA}}{Hierarchical Recurrent Encoder with Attention}

\nomenclature[A]{\textbf{KVQA}}{Knowledge-aware Visual Question Answering}

\nomenclature[A]{\textbf{LBA}}{Learning-By-Asking}
\nomenclature[A]{\textbf{LF}}{Late Fusion}
\nomenclature[A]{\textbf{LGCN}}{Language-Conditioned Graph Networks}
\nomenclature[A]{\textbf{LSTM}}{Long Short-Term Memory}
\nomenclature[A]{\textbf{LXMERT}}{Learning Cross-Modality Encoder Representations from Transformers}

\nomenclature[A]{\textbf{MAC}}{Memory, Attention, and Composition} 
\nomenclature[A]{\textbf{MedRank}}{Median Rank}
\nomenclature[A]{\textbf{METEOR}}{Metric for Evaluation of Translation with Explicit Ordering}
\nomenclature[A]{\textbf{MIL}}{Multiple Instance Learning}
\nomenclature[A]{\textbf{MMT}}{Multimodal Machine Translation}
\nomenclature[A]{\textbf{MN}}{Memory Network}
\nomenclature[A]{\textbf{MPII}}{Max Planck Institute for Informatics}
\nomenclature[A]{\textbf{MPII-MD}}{MPII Movie Description}
\nomenclature[A]{\textbf{MRR}}{Mean Reciprocal Rank}
\nomenclature[A]{\textbf{MSCOCO}}{Microsoft Common Objects in COntext}
\nomenclature[A]{\textbf{MSR-VTT}}{Microsoft Research Video to Text}
\nomenclature[A]{\textbf{MSVD}}{Microsoft Video Description}
\nomenclature[A]{\textbf{MuRel}}{Multimodal Relational network}
\nomenclature[A]{\textbf{M-VAD}}{Montreal Video Annotation}

\nomenclature[A]{\textbf{NDCG}}{Normalized Discounted Cumulative Gain}
\nomenclature[A]{\textbf{NIC}}{Neural Image Captioning}
\nomenclature[A]{\textbf{NMT}}{Neural Machine Translation}
\nomenclature[A]{\textbf{NS-CL}}{Neuro-Symbolic Concept Learner}
\nomenclature[A]{\textbf{NYC-Storytelling}}{New York City Storytelling}

\nomenclature[A]{\textbf{OK-VQA}}{Outside Knowledge Visual Question Answering}
\nomenclature[A]{\textbf{OSCAR}}{Object-SemantiCs Aligned pRe-training}

\nomenclature[A]{\textbf{PPGN}}{Plug \& Play Generative Network}

\nomenclature[A]{\textbf{R2R}}{Room-2-Room}
\nomenclature[A]{\textbf{RAVEN}}{Relational and Analogical Visual rEasoNing}
\nomenclature[A]{\textbf{RCM}}{Reinforced Cross-modal Matching}
\nomenclature[A]{\textbf{R-CNN}}{Region-based CNN}
\nomenclature[A]{\textbf{RE}}{Referring Expression}
\nomenclature[A]{\textbf{RGB-D}}{Red, Green, Blue, Depth}
\nomenclature[A]{\textbf{RL}}{Reinforcement Learning}
\nomenclature[A]{\textbf{RNs}}{Relation Networks}
\nomenclature[A]{\textbf{ROUGE}}{Recall Oriented Understudy for Gisting Evaluation}
\nomenclature[A]{\textbf{RvA}}{Recursive Visual Attention}

\nomenclature[A]{\textbf{SCA}}{Sequential Co-Attention}
\nomenclature[A]{\textbf{SCRC}}{Spatial Context Recurrent Convnet}
\nomenclature[A]{\textbf{SDR}}{Spatial Description Resolution}
\nomenclature[A]{\textbf{SF}}{Similarity scoring + Fusion}
\nomenclature[A]{\textbf{SGD}}{Stochastic Gradient Descent}
\nomenclature[A]{\textbf{SIL}}{Self-supervised Imitation Learning}
\nomenclature[A]{\textbf{SIS}}{Stories for Images-in-Sequence}
\nomenclature[A]{\textbf{SIND}}{Sequential Image Narrative Dataset}
\nomenclature[A]{\textbf{SPICE}}{Semantic Propositional Image Captioning Evaluation}

\nomenclature[A]{\textbf{TACoS}}{Textually Annotated Cooking Scenes}

\nomenclature[A]{\textbf{UNITER}}{UNiversal Image-TExt Representation Learning}

\nomenclature[A]{\textbf{VATEX}}{Video And TEXt}
\nomenclature[A]{\textbf{VDG}}{Visual Description Generation}
\nomenclature[A]{\textbf{VGG}}{Visual Geometry Group}
\nomenclature[A]{\textbf{VIST}}{Visual Storytelling}
\nomenclature[A]{\textbf{VLN}}{Vision and Language Navigation}
\nomenclature[A]{\textbf{VLP}}{Vision-Language Pre-training}
\nomenclature[A]{\textbf{VMMT$_F$}}{Variational MMT with Fixed Gaussian prior}
\nomenclature[A]{\textbf{VRE}}{Visual Referring Expression}
\nomenclature[A]{\textbf{V-SNLI}}{Visually-grounded Natural Language Inference}
\nomenclature[A]{\textbf{VTW}}{Videos Titles in the Wild}

%\nomenclature[N]{$c$}{speed of light in vacuum}
%\nomenclature[N]{$h$}{Plank constant}

\printnomenclature[2cm]
